# Supplementary material for: Planar Robot Casting with Real2Sim2Real Self-Supervised Learning
Source: arXiv:2111.04814 source file (2022-06-25)
Supplement: Supplementary file 1 [file appendix.tex]

%%%%%%%%%%%%
% APPENDIX %
%%%%%%%%%%%%
\section{Appendix}\label{app}
The appendix is structured as follows:

\begin{itemize}
    \item In Appendix~\ref{app:isaac-gym} we provide more background on NVIDIA Isaac Gym 
    \item In Appendix~\ref{app:method-details} we provide more details on the methodology.
\end{itemize}

\subsection{NVIDIA Isaac Gym}\label{app:isaac-gym}

We use the Flex physics engine in Isaac Gym. With the Flex backend, we use the Newton Jacobi solver for its determinism guarantees to ensure consistent Real2Sim tuning results. We use a simulation timestep of 1/60\,s with 8 substeps, 5 inner iterations, and 20 outer iterations, and did not observe these parameters to affect the determinism. However, we observed that increasing the granularity of these parameters to increase simulation stability and fidelity results in substantially increased runtime. As such, we minimized these parameters to the extent permitting stability.

For the Isaac Gym segmented model, the cable has 18 rigid links connected by ball joints. We tried increasing the number of links up to a maximum of 30 and noticed insignificant increase in simulation fidelity, but a significant decrease in simulation fidelity. As the rigid links are connected by ball joints, the segmented model should be unable to model stretching along the length of the cable. However, we noticed stretching along the length of the cable in as we increased the number of rigid links, which we interpreted as a sign of simulation instability and opted to decrease the number of rigid links.  

\subsection{Additional Method Details}\label{app:method-details}

For policy $\pireal$, we parameterize the forward dynamics model $f_{\rm forw}$ with a feedforward neural network with 3 layers, each with 32 hidden units, and mini-batch size of 16. For policies $\pisim$ and $\pitune$, we parameterize $f_{\rm forw}$ with a larger neural network with 3 layers, each with 128 hidden units, and a mini-batch size of 64. We use a smaller neural network for $\pireal$ to avoid overfitting to the small real dataset, whereas $\pisim$ and $\pitune$ both train on larger, more diverse datasets. For all policies, we use the Adam optimizer~\cite{adam2015} and a learning rate of $10^{-3}$.

For each policy, we train the neural network to minimize the predicted $L^2$ loss for each $(\ba, \bs)$ data sample. For $\pisim$, we weight $\dreal$ samples 2$\times$ higher for cable 1, and 3$\times$ higher for cable 2, and $2\times$ higher for cable 3. We additionally tested upsampling percentages of between 20\% and 50\%, and picked values between 30\% and 40\%. These hyperparameters were chosen empirically to maximize performance. 

For grid sampling of the five trajectory parameters, the bounds for $\dreal$ are shown in Table~\ref{tab:dphys_samp}. The bounds were chosen to empirically maximize coverage of the reachable workspace.

\begin{table}[H]
  \setlength\tabcolsep{5.0pt}
  \centering
  \normalsize
  \begin{tabular}{@{}lccc@{}}
  \toprule
  Parameter & Lower & Upper & Frequency \\
  \midrule
  $\theta_1$ & \ang{1} & \ang{80} & 5 \\
  $\theta_2$ & \ang{20} & \ang{80} & 5 \\
  $r_2$ & 0.21 & 0.77 & 5 \\
  $\alpha$ & \ang{30} & \ang{60} & 4 \\
  $\vmax$ & 2 & 2.5 & 2 \\
  \toprule
  \end{tabular}
  \caption{$\dreal$ grid sampling ranges.}
  \label{tab:dphys_samp}
\end{table}

The grid sampling bounds for $\dsim$ is similar, with the only difference being the sampling frequency and the bounds for $\theta_2$, as shown in Table~\ref{tab:dsim_samp}.

\begin{table}[H]
  \setlength\tabcolsep{5.0pt}
  \centering
  \normalsize
  \begin{tabular}{@{}lccc@{}}
  \toprule
  Parameter & Lower & Upper & Frequency \\
  \midrule
  $\theta_1$ & \ang{1} & \ang{80} & 15 \\
  $\theta_2$ & \ang{1} & \ang{80} & 15 \\
  $r_2$ & 0.21 & 0.77 & 15 \\
  $\alpha$ & \ang{30} & \ang{60} & 5 \\
  $\vmax$ & 2 & 2.5 & 2 \\
  \toprule
  \end{tabular}
  \caption{$\dsim$ grid sampling ranges.}
  \label{tab:dsim_samp}
\end{table}

For tuning with Differential Evolution, we use the default parameters as implemented by SciPy~\cite{2020SciPy-NMeth}.

\subsection{Cable Model Parameters} \label{app:cable}

\Vincent{TODO}
